# Supplementary material for: Extracting Social Determinants of Health from Pediatric Patient Notes Using Large Language Models: Novel Corpus and Methods
Source: arXiv:2404.00826 source file (2024-04-04)
Supplement: Supplementary file 1 [file 8_appendix.tex]

% \begin{table*}[ht]
% \centering
% \small
% \input{tables/annotator_agreement}
% \caption{Annotator agreement}
% \label{ann_guideline}
% \end{table*}
